# Supplementary material for: Degenerate Feedback Loops in Recommender Systems
Source: arXiv:1902.10730 source file (2019-03-27)
Supplement: Supplementary file 1 [file appendix.tex]

\begin{appendices}
{\todo fix appendix citation and title}

\section{Proofs of theorems}
\label{proofs}
\addtocounter{theorem}{-7}
 \subsection{Proof of Theorem~\ref{thm:s1_suff}}
 
 \begin{lemma}
 Let $\s$ be a finite set of options. If at least $k$ distinct elements are served from $\s$ every time step, then at least $k$ elements from $\s$ are served infinitely often.
 \label{lem:s11}
 \end{lemma}
 \begin{proof}
 Suppose the contrary is true. There are $k'$ elements served infinitely often and $k'<k$. Without loss of generality, let this set be $\{1, 2, \ldots k'\}$ or $[k']$. Let $m$ be the maximum number of times any element is served from $\s\setminus[k']$. Since at least $k$ distinct elements are served from $\s$ every time step, then at least $k-k'$ elements served are from the set $\s\setminus[k']$. The total number of service times from this set is at most $m\cdot|\s| < \infty$. However $(k-k')t\rightarrow \infty$ as $t\rightarrow\infty$. This is a contradiction! 
 \end{proof}
 
 \begin{lemma}
Let $\s$ be a finite set of options. Let $d$ be an integer such that $0 < d \leq |\s|$. Using definitions from Theorem~\ref{thm:s1_suff}, if $\exists a^1, a^2, \ldots, a^d\in\s$ such that as $t\rightarrow\infty, \mu_t(a^i) \rightarrow \infty$, for $i=1,2\ldots,d$, and any other $a$ has bounded values of $\mu_t(a)$, i.e. for any other $a\in\s$, $\exists B>0$ s.t. $\mu_t(a)<B$ for any $t$. Then given any $t_0>0$, there must exist a time $t'>t_0$ such that $\theta_{t'}(a^1), \ldots, \theta_{t'}(a^d)$ constitute the top $d$ values of $\theta_{t'}(a)$ for $a\in\s$.
\label{lem:s12}
\end{lemma}

\begin{proof}
We argue by contradiction. Define the set of options $\A=\{a^1, a^2, \ldots, a^d\}$. Suppose the contrary is true, i.e. $\exists t_0>0$ such that for $\forall t\geq t_0, \exists a_t\in\s\setminus\A$ such that $\theta_t(a_t)$ is in the top $d$ values. Since $|\s|$ is finite whereas the sequence $\{a_{t_0}, a_{t_0+1}, \ldots\}$ is infinite, there must exist an option $a^*$ where $\theta_t(a^*)$ is in the top $d$ values for infinitely many times after time $t_0$. Thus there exists an infinite sequence $\{t_1, t_2, \ldots\}$ where $\theta_{t_i}(a^*) > \theta_{t_i}(a^{j_t})$ for some $j_t\in[d]$. Hence $\theta_{t_i}(a^*) > \theta_{t_i}(a^{j_t}) > \min_{i\in[d]}(\theta_{t_i}(a^i))$. Since $\mu_t(a^i) \rightarrow \infty$ as $t \rightarrow \infty$ for any $i=1,2\dots,d$, we have $\theta_t(a^i) \rightarrow \infty$ as $t \rightarrow \infty$  due to Condition~\ref{eq:_bdd_s1}. Since $d$ is finite, $\min_{i\in[d]}(\theta_{t_i}(a^i))\rightarrow \infty$ as $t\rightarrow \infty$ as well. Thus so do $\theta_{t_i}(a^*)$ and $\mu_{t_i}(a^*)$ by Condition~\ref{eq:_bdd_s1}. This is a contradiction with the assumption that any $a\in\s\setminus\A$ must have bounded $\mu_t(a)$.
\end{proof}

\addtocounter{theorem}{-2}
\begin{theorem}
Let $\mu_t, \theta_t:[m]\rightarrow \mathbb{R}$. Let $D\in\mathbb{R}$. If the following conditions hold,
\begin{align}
    &a^1_t, a^2_t, \ldots a^k_t = \text{ top k } (\theta_t(a)),\label{eq:_opt_s1}\\
    &c_t(a) = (\mu_t(a)>D), \text{ for } \forall a\in [m],\\
    &c_t(a) = 1 \Leftrightarrow
    \begin{cases}
        \theta_{t+1}(a) > \theta_t(a), \label{eq:_pos_reinforce1_s1}\\
        \mu_{t+1}(a) > \mu_t(a).
    \end{cases}\\
    &c_t(a) = 0 \Leftrightarrow
    \begin{cases}
        \theta_{t+1}(a) < \theta_t(a), \label{eq:_pos_reinforce2_s1}\\
        \mu_{t+1}(a) < \mu_t(a).
    \end{cases}\\
    &\forall t_0 > 0, \forall a\in[m] \text{ where } |\{t|a_t=a\}|=\infty,\notag\\ 
    &\qquad \sum_{\substack{t=t_0, \\a_t=a}}^\infty |\mu_{t+1}(a) - \mu_t (a)| = \infty,\label{eq:_inf_s1}\\
    &\exists B>0, \text{ s.t. for } \forall t>0, \forall a\in[m], \notag\\
    &\qquad |\theta_t(a) - \mu_t(a)|<B, \label{eq:_bdd_s1}
\end{align}
then we have a degenerate system, that is, $\lim_{t\rightarrow \infty}\|\mu_t - \mu_0\|_p = \infty$. Specifically, as $t \rightarrow \infty$, the system results in either of the two following scenarios.
\begin{enumerate}
    \item $\mu_t(a^i) \rightarrow \infty$ for $k$ elements $a^i\in[m]$,
    \item Strictly less than $k$ elements have $\mu_t(a^i) \rightarrow \infty$. For any other $a\in [m]$, $\mu_t(a)\rightarrow -\infty$ as $i\rightarrow \infty$.
\end{enumerate}  
\end{theorem}
\begin{proof}
In the first scenario, we argue by contradiction. Suppose $\exists a^1, a^2, \ldots, a^{k'}\in[m]$ such that $\mu_t(a^i)\rightarrow\infty$ as $t\rightarrow\infty$, that is, $\forall N>0, \exists t_0>0$ s.t. $\mu_t(a^i)>N$ for all $t \geq t_0, i=[1,\ldots,k']$ and $k'>k$. Pick $N>D$. Moreover any $a\in[m]\setminus[k']$ has bounded $\mu_t(a)$. Invoking Lemma~\ref{lem:s12}, $\exists t'>t_0$ s.t. $\theta_{t'}(a^i)$ are the top $k'$ values for $i=1,2\dots,k'$. Without loss of generality, let $a^1,\ldots, a^{k'}$ be a decreasingly sorted list according to values of $\theta_{t'}(a^i)$. Since the system can only select $k$ options at time $t'$, it selects $a^1, \ldots, a^k$. Since $N>D$, we have $c_{t'}(a^i)=1$ for $i=1,\ldots,k$. Hence all top $k$ values of $\theta_t(a^i)$ increase and they remain in the top $k$ for time $t'+1$. Iterate the same argument for $t=t'+2, t'+3, \ldots$ and we conclude that $a^{k+1}, \ldots, a^{k'}$ will not be selected after $t'$. This contradicts with $\mu_t(a^i)\rightarrow \infty$ as $t\rightarrow \infty$ for $i=k+1, \ldots, k'$! 

In the second scenario, suppose there are strictly less than $k$ elements with $\mu_t(a)\rightarrow\infty$. Let these elements be $a^1, a^2, \ldots, a^{k'}\in[m]$ and $k'<k$. For all $a\in[m]\setminus[k']$, $\mu_t(a)$ is bounded, that is, $\exists N_0>0$ such that $\forall t_0>0$, we have $\mu_t(a)<N_0$ for $\forall t\geq t_0$. Since at least $k-k'$ distinct options are served from the set $[m]\setminus [k']$ at every time step, by Lemma~\ref{lem:s11} we conclude at least $k-k'$ distinct options from $[m]\setminus[k']$ are served infinitely many times. Call this set $\h$. For $\forall a\in\h$, we discuss the following three cases based on values of the feedback $c_t(a)$.
\begin{enumerate}
    \item $c_t(a) = 0$ infinitely often, $c_t(a) = 1$ finitely often. Thus $\exists t_m$ such that $c_t(a)=0$ for all $t>t_m$. By Condition~\ref{eq:_inf_s1}, we have
    \begin{align}
     &\sum_{\substack{t=t_m, \\a_t=a, \\c_t(a)=0}}^\infty |\mu_{t+1}(a) - \mu_t (a)| \\
     =& \sum_{\substack{t=t_m, \\a_t=a}}^\infty |\mu_{t+1}(a) - \mu_t (a)| = \infty.
    \end{align}
    Due to Condition~\ref{eq:_pos_reinforce2_s1}, in this case $\mu_t(a)\rightarrow -\infty$ as $t\rightarrow \infty$.
    \item $c_t(a) = 1$ infinitely often, $c_t(a) = 0$ finitely often. This case is the opposite of Case 1. We follow the same argument above and conclude $\mu_t(a)\rightarrow\infty$ as $t\rightarrow\infty$, which contradicts with the assumption that $\forall a\in\h\subset[m]\setminus[k']$ has bounded $\mu_t(a)$.
    \item $c_t(a) = 1$ and $c_t(a) = 0$ infinitely often. This requires $\mu_t(a)$ to move above and below the threshold $D$ infinitely often. Suppose at some time $\mu_{t_0}(a)<D$, then $c_{t_0}(a)=0$. Thus $\mu_{t_0+1}(a)<\mu_{t_0}(a)<D$. When $a$ is selected again at $t'$, we have $c_{t'}(a)=0$ and $\mu_{t'}(a)$ will decrease again. $\mu_{t'}(a)$ can never move above $D$ again. This argument applies for the opposite case $\mu_{t_0}(a)>D$ as well. Thus this is an impossible case.
\end{enumerate}
Therefore, only Case 1 is possible. For $\forall a^*\in\h$, $\mu_t(a^*)\rightarrow -\infty$ as $t\rightarrow \infty$. Since $|\theta_t(a^*) - \mu_t(a^*)|<B$ (Condition~\ref{eq:_bdd_s1}), $\theta_t(a^*)\rightarrow -\infty$ as $t\rightarrow \infty$. For $\forall a\in [m]\setminus([k']\cup\h)$, option $a$ has been selected at most finite number of times. Thus $\exists t_a$ such that option $a$ is never selected after $t_a$ and $\theta_t(a)\equiv\theta_{t_a}(a)$. This contradicts with $\theta_{t_i}(a) < \theta_{t_i} (a^*)\rightarrow -\infty$ as $i\rightarrow \infty$ where $\{t_1, t_2\ldots\}, t_1>t_a,$ is the infinite sequence of time steps when $a^*$ is selected. Therefore $[m]\setminus([k']\cup\h) = \emptyset$, or $[m] = [k']\cup\h$.
\end{proof}

\subsection{Proof of Theorem~\ref{thm:s2_suff}}
{\todo Specify in every proof whenever a condition in the theorem is used.}

\begin{lemma}
Let $d$ be a positive integer. Using definitions from Theorem~\ref{thm:s3_suff}, if $\exists a^1, a^2, \ldots, a^d\in\M$ s.t. $\mu_t(a^i) \rightarrow \infty$ as $t \rightarrow \infty$ for $i=1,2\ldots,d$, and for any other $a\in\M$, $\exists B>0$ s.t. $\mu_t(a)<B$ for any $t$. Then for any $t_0>0$ there must exist a time $t'>t_0$ such that $\theta_{t'}(a^1), \ldots, \theta_{t'}(a^d)$ constitute the top $d$ values of $\theta_{t'}(a)$ for $a\in\s_{t'}$.
\label{lem:s3}
\end{lemma}
\begin{proof}
Since $\mu_t(a^i) \rightarrow \infty$ as $t \rightarrow \infty$ for any $i=1,2\ldots,d$ and $d<\infty$, then it means that for any $N>0$, $\exists t_0$ s.t. for $\forall t>t_0$, we have $\mu_t(a^i)>N$. Take $N>C$ for $C$ defined in Theorem~\ref{thm:s3_suff}. Then we have $\mu_t(a^i)>N>C$. This means that for $\forall t>t_0$, the top k options at time $t$ can only be selected from $\s_{t_0}$ due to Condition~\ref{eq:_bdd_init}, which is a finite set of options containing $a^1, a^2, \ldots, a^d$. Therefore by Lemma~\ref{lem:s2}, for any $t_0>0$ there must exist a time $t'>t_0$ such that $a^1, \ldots, a^d$ constitute the top $d$ values of $\theta_{t'}(a)$ for $a\in\s_{t_0}\subset\s_{t'}$. 
\end{proof}

\addtocounter{theorem}{-1}

\begin{theorem}
Let $\mu_t, \theta_t:\s_t\rightarrow \mathbb{R}$. Let $\phi:\mathbb{R}\rightarrow[0,1]$ be any non-decreasing surjective function. If the following conditions hold,
\begin{align}
    &a^1_t, \ldots, a^k_t = \text{ top k } (\theta_t(a)),\\
    &\text{ where }a\in\s_t, \s_{t-1}\subset\s_t\subset \M, |\s_t|<\infty,\label{eq:_subset}\\
    &\exists C>0, \text{ s.t. } \theta_t(a)<C, \text{ for }\forall a\in\s_t\setminus\s_{t-1},\label{eq:_bdd_init}\\
    &\exists \text{ a non-empty } \h\subset\M \text{ such that}\\
    &\qquad \forall a\in\h \text{ is served infinitely often},\\ 
    &c_t(a) = Bernoulli(p=\phi(\mu_t(a))), \forall a\in \M,\\
    &c_t(a) = 1: 
    \begin{cases}
        \theta_{t+1}(a) > \theta_t(a), \\
        \mu_{t+1}(a) > \mu_t(a).
    \end{cases}\\
    &c_t(a) = 0:
    \begin{cases}
        \theta_{t+1}(a) < \theta_t(a), \\
        \mu_{t+1}(a) < \mu_t(a).
    \end{cases}\\
    &\forall t_0 > 0, \forall a\in\M, s.t. |\{t|a_t=a\}|=\infty,\notag\\ 
    &\qquad \sum_{\substack{t=t_0, \\a_t=a}}^\infty |\mu_{t+1}(a) - \mu_t (a)| = \infty,\\
    &\exists B>0, \text{ s.t. for } \forall t>0, \forall a\in\M, |\theta_t(a) - \mu_t(a)|<B,
\end{align}
then we have a degenerate system, specifically the system results in either of the two following scenarios.
\begin{enumerate}
    \item $\mu_t(a^i) \rightarrow \infty$ with probability 1 for $1$ to $k$ elements $a^i\in\M$,
    \item $\mu_t(a^i) \rightarrow -\infty$ for $\forall a \in\h$. For $\forall a\in\mathcal{M}\setminus\h$, there exists an infinite sequence $\{t_1, t_2, \ldots\}$ where $\mu_{t_i}(a)\rightarrow -\infty$ as $i\rightarrow \infty$. 
\end{enumerate}  
\end{theorem}

\begin{proof}
We argue by contradiction. Suppose $\exists a^1, a^2, \ldots, a^{k'}\in\M$ s.t. for $\forall N>0, \exists t_0>0$ s.t. $\mu_t(a^i)>N$ for all $t \geq t_0, i=[1,\ldots,k']$ and $k'>k$. Take $N'>C+B$ and let $t'_0$ be the corresponding $t_0$. All other $a\in\M$ have bounded $\mu_t(a)$ for any $t>0$. Invoking Lemma~\ref{lem:s3}, $\exists t'>t'_0$ s.t. $\theta_{t'}(a^i)$ are the top $k'$ values in $\s_{t'}$ for $i=1,2\dots,k'$. Without loss of generality, let $a^1,\ldots, a^{k'}$ be a decreasingly sorted list according to values of $\theta_{t'}(a^i)$. Since the system can only select $k$ options at time $t'$, it selects $a^1, \ldots, a^k$. Since $N'$ can be arbitrarily large, with probability 1 we have $c_{t'}(a^i)=1$ for $i=1,\ldots,k$. Hence the top $k$ values of $\theta_{t'}(a^i)$ all increase at $t'+1$. 

At $t'+1$, we have 
\[
\mu_{t'+1}(a^i) > N' > C+B > \theta_{t'+1}(a)+B > \mu_{t'+1}(a),
\] 
for $i=1,\ldots,k$ and $a\in\s_{t'+1}\setminus\s_{t'}$. For all other $a\in\s_{t'}$, $\theta_{t'+1}(a) = \theta_{t'}(a)$, thus remaining the same. Notice that this is true for all $t>t'$. By inferring on every time step, they maintain in the top $k$ of $\s_{t}$ for $t>t'$. Therefore $a^{k+1}, \ldots, a^{k'}$ will be selected after time $t'$ with probability 0. This is a contradiction with $\mu_t(a^i)\rightarrow \infty$ as $t\rightarrow \infty$ for $i=k+1, \ldots, k'$! 

Now if for $\forall a\in\M$, $\theta_t(a)$ is always bounded from above. Then for $\forall a\in\h$, by the same argument as in the proof of Theorem~\ref{thm:s1_suff}, we have $c_t(a)=0$ for infinitely many times $t$. Thus we conclude that $\mu_t(a)\rightarrow-\infty$ as $t\rightarrow\infty$. For $\forall a\in\mathcal{M}\setminus\h$, since it can only be selected finitely many times, by the same argument as in Theorem~\ref{thm:s1_suff} again, we conclude that for $\forall a\in\mathcal{M}\setminus\h$, there exists an infinite sequence $\{t_1, t_2, \ldots\}$ where $\mu_{t_i}(a)\rightarrow -\infty$ as $i\rightarrow \infty$. 
\end{proof}

\subsection{Proof of Theorem~\ref{thm:s3_suff}}
\addtocounter{theorem}{-1}

\begin{lemma}
If $d(\theta^i_t, \theta^j_t) < \epsilon$, then $|\theta^i_t(a) - \theta^j_t(a)| < \epsilon$ for all $a\in \s_t$.
\label{lem:s41}
\end{lemma}
\begin{proof}
For $\forall a\in \s_t$, $|\theta^i_t(a) - \theta^j_t(a)| = |\theta^i_t(a) - \theta^j_t(a)|^{p\cdot\frac{1}{p}}\leq \left(\sum_{a\in\s_t} |\theta^i_t(a) - \theta^j_t(a)|^p\right)^{\frac{1}{p}} < \epsilon.$
\end{proof}

\begin{theorem}
Let $n$ be a positive integer. Consider a user $i\in[n]$. We denote variables for user $i$ by superscript $i$. Let $\mu^i_t, \theta^i_t:\s_t\rightarrow \mathbb{R}$ for $i\in[n]$. Let $\phi:\mathbb{R}\rightarrow[0,1]$ be any non-decreasing surjective function. Let $\epsilon\in\mathbb{R}^+$. Define the influence set of users $\U_i$ to user $i$, $\U^i_t:=\{u\in[n] \mid d(\theta^i_t, \theta^u_t)<\epsilon\}$. If the following conditions hold,

\begin{align}
    &a^{1, i}_t, \ldots, a^{k, i}_t = \text{ top k } (\theta^i_t(a)), \\
    &\text{ where } a\in\s_t, \s_{t-1}\subset\s_t\subset \M, |\s_t|<\infty, \forall i\in[n],\\
    &\exists C>0, \text{ s.t. } \theta^i_t(a)<C, \text{ for }\forall a\in\s_t\setminus\s_{t-1},  \forall i\in[n],\label{eq:_bdd_init_u}\\
    &\forall i\in[n], \exists \text{ a non-empty } \h^i\subset\M \text{ such that}\\
    &\qquad \forall a\in\h^i \text{ is served infinitely often},\\ 
    &c^i_t(a) = Bernoulli(p=\phi(\mu^i_t(a))), \forall a\in \M,  \forall i\in[n],\\
    &c^i_t(a) = 1: 
    \begin{cases}
        \theta^i_{t+1}(a) > \theta^i_t(a), \\
        \theta^j_{t+1}(a) > \theta^j_t(a) \text{ for } \forall j\in\U^i_t,\\
        \mu^i_{t+1}(a) > \mu^i_t(a).
    \end{cases}\\
    &c^i_t(a) = 0:
    \begin{cases}
        \theta^i_{t+1}(a) < \theta^i_t(a), \\
        \theta^j_{t+1}(a) < \theta^j_t(a) \text{ for } \forall j\in\U^i_t,\\
        \mu^i_{t+1}(a) < \mu^i_t(a).
    \end{cases}\\
    &|\theta^i_{t+1}(a^{l, i}_t) - \theta^i_t(a^{l, i}_t)| > \sum_{u\in\U^i_t} |\theta^i_{t+1}(a^{l', u}_t) - \theta^i_t(a^{l', u}_t)|, \\
    &\text{ for } l,l'\in[k].\label{eq:_direct_influence_u}\\
    &\forall t_0 > 0, \forall j\in[n], \forall a\in\M, s.t. |\{t|a_t=a\}|=\infty,\notag\\ 
    &\qquad \sum_{\substack{t=t_0, \\a_t=a}}^\infty |\mu^j_{t+1}(a) - \mu^j_t (a)| = \infty,\\
    &\exists B>0, \text{ s.t. for } \forall t>0, \forall a\in\M, \\
    &\qquad|\theta^i_t(a) - \mu^i_t(a)|<B,  \forall i\in[n],\label{eq:_bdd_est_u}
\end{align}
then we have a degenerate system, specifically the system results in either of the two following scenarios. For any user $j\in[n]$,
\begin{enumerate}
    \item $\mu^j_t(a) \rightarrow \infty$ with probability 1 for $1$ to $k$ elements $a\in\M$,
    \item $\mu^j_t(a) \rightarrow -\infty$ for $\forall a \in\h^j$. For $\forall a\in\mathcal{M}\setminus\h^j$, there exists an infinite sequence $\{t_1, t_2, \ldots\}$ where $\mu^j_{t_i}(a)\rightarrow -\infty$ as $i\rightarrow \infty$. 
\end{enumerate} 
\end{theorem}
\begin{proof}
We argue by contradiction. Let $j\in[n]$ be any user. Suppose the contrary to the conclusion, i.e. $\exists a^1, a^2, \ldots, a^{k'}\in\M$ s.t. for $\forall N>0, \exists t_0>0$ s.t. $\mu^j_t(a^i)>N$ for all $t \geq t_0, i=[1,\ldots,k']$ and $k'>k$. Take $N'>C+B$ and let $t'_0$ be the corresponding $t_0$. All other $a\in\M$ have bounded $\mu^j_t(a)<B_m$ for any $t>0$. Invoking Lemma~\ref{lem:s3}, $\exists t'>t'_0$ s.t. $\theta^j_{t'}(a^i)$ are the top $k'$ values in $\s_{t'}$ for $i=1,2\dots,k'$. Without loss of generality, let $a^1,\ldots, a^{k'}$ be a decreasingly sorted list according to values of $\theta^j_{t'}(a^i)$. Since the system can only select $k$ options at time $t'$, it selects $a^1, \ldots, a^k$. Since $N'$ can be arbitrarily large, with probability 1 we have $c^j_{t'}(a^i)=1$ for $i=1,\ldots,k$. 

The distance measure $d$ is symmetric, i.e. $d(\mu^i_t, \mu^j_t) = d(\mu^j_t, \mu^i_t)$. Then $\U^j_t$ contains all the users that may change $\theta^j_t$. By Lemma~\ref{lem:s41}, for any $u\in\U^j_t$ we have $|\theta^u_t(a) - \theta^j_t(a)| < \epsilon$ for all $a\in \s_t$. Thus if we consider the model update equations for user $u$, and let $N^u = N'-\epsilon-2B$, then 
\begin{align}
&\mu^u_t(a^i) > \theta^u_t(a^i)-B > (\theta^j_t(a^i)-\epsilon)-B \\
&> (\mu^j_t(a^i)-B)-\epsilon-B > N'-\epsilon-2B = N^u,
\end{align}
for all $t \geq t'_0, i=[1,\ldots,k']$. Thus $\mu^u_t(a)\rightarrow \infty$ as $t\rightarrow\infty$ for $u\in\U^j_t, i=[1,\ldots,k']$. For all other options $a\in\M$, $\mu^u_t(a)$ must be bounded by $B_m+\epsilon+2B$ for all $t>0$. Invoking Lemma~\ref{lem:s3} again, $\exists t'>t'_0$ s.t. $\theta^u_{t'}(a^i)$ are the top $k'$ values in $\s_{t'}$ for $i=1,2\dots,k'$. The system selects the top $k$ values for user $u$ at time $t'$. Let the top $k$ options be $a^{\pi_1}, \ldots, a^{\pi_k}$. Since $N^u$ can be arbitrarily large, $c^u_{t'}(a^{\pi_i})=1$ with probability 1. Thus any user activity from the influence set $\U_j$ does not decrease any model parameter $\theta^j_t$ for user $j$.

Hence the top $k$ values of $\theta^j_{t'}(a^i)$ all increase at $t'+1$. We look at whether the top $k$ options can change in the next step by examining the model parameters for all options in $\s_{t'+1}$. Notice that 
\[
\s_{t'+1} = (\s_{t'+1}\setminus\s_{t'}) \cup (\s_{t'}\setminus[k']) \cup ([k']\setminus[k]) \cup [k].
\] 
At $t'+1$, we have 
\[
\mu^j_{t'+1}(a^i) > N' > C+B > \theta^j_{t'+1}(a)+B > \mu^j_{t'+1}(a),
\] 
for $i=1,\ldots,k$ and $a\in\s_{t'+1}\setminus\s_{t'}$. Since for $\forall u\in\U_j$, only $a^1, \ldots, a^{k'}$ are possible to be selected. The model parameters $\theta^j_{t'+1}(a), a\not\in[k']$ won't be affected by other users. Hence for all other $a\in\s_{t'}\setminus[k']$, $\theta^j_{t'+1}(a) = \theta^j_{t'}(a)$, remaining the same. The only options that may be listed into the top $k$ at time $t'+1$ are $a^1, \ldots, a^{k'}$. However from Condition~\ref{eq:_direct_influence_u}, for any $a^l, l=k+1, \ldots, k'$ that is served to any users $u\in\U^j_t$, $\Delta \theta^j_{t'}(a^i) > \sum_u \Delta \theta^j_{t'}(a^l)$ for $i=1,\ldots, k$. Thus $\theta^j_{t'+1}(a^l), l=k+1, \ldots,k'$ are smaller than any of $\theta^j_{t'+1}(a^i), i=1, \ldots, k$. The top $k$ options remain $a^1, \ldots, a^k$. Notice that the analysis is true for all $t>t'$. 

Therefore by inferring on every time step, $a^1, \ldots, a^k$ maintain in the top $k$ options of $\s_{t}$ for $t>t'$. Therefore $a^{k+1}, \ldots, a^{k'}$ will be selected after time $t'$ with probability = 0. This is a contradiction with $\mu^j_t(a^i)\rightarrow \infty$ as $t\rightarrow \infty$ for $i=k+1, \ldots, k'$! 

In the second scenario, with Condition~\ref{eq:_direct_influence_u} we can apply the same argument as in Theorem~\ref{thm:s2_suff} for each user $j\in[n]$, and reach the stated conclusion. {\todo double check carefully}
\end{proof}

\section{Summary of essential sufficient conditions}
\label{essential_suff}
Notice that Theorem~\ref{thm:s1_suff}-\ref{thm:s3_suff} still hold when we restrict the codomain of the function $\mu_t$ to a finite range $\mathcal{D}$ by simply replacing $\mu_t$ with $\psi(\mu_t)$ where $\psi:\M\rightarrow \mathcal{D}$. Thus some of the conditions in the sufficiency theorems are useful for derivation of their proofs but may not provide intuition for the main causes of degeneracy in a control system. Below we recall and summarize the essential conditions in each theorem, and their interpretation in practice.
\begin{enumerate}
    \item Essential conditions in Theorem~\ref{thm:s1_suff}:
        \begin{flalign*}
        &a_t = \argmax_a \theta_t(a),\\
        &\text{(The system optimizes for user feedback.)}\\
        &c_t = 1: 
        \begin{cases}
            \theta_{t+1}(a_t) > \theta_t(a_t), \\
            \mu_{t+1}(a_t) > \mu_t(a_t). 
        \end{cases}\\
        &c_t = 0:
        \begin{cases}
            \theta_{t+1}(a_t) < \theta_t(a_t), \\
            \mu_{t+1}(a_t) < \mu_t(a_t). 
        \end{cases}\\
        &\text{(Model estimate and user interest for an engaged option }\\
        &\text{increase, and vice versa.) }\\ 
        &\exists B>0, \text{ s.t. for } \forall t>0, \forall a\in[m], |\theta_t(a) - \mu_t(a)|<B, \\
        &\text{(Model estimates cannot be completely inaccurate.) }
        \end{flalign*}
    \item Theorem~\ref{thm:s2_suff} is very similar to Theorem~\ref{thm:s1_suff} but just for top $k$ items.
    \item New conditions in Theorem~\ref{thm:s3_suff}:
        \begin{flalign*}
        &a^1_t, \ldots, a^k_t = \text{ top k } (\theta_t(a)), \\
        &\text{ where }a\in\s_t, \s_{t-1}\subset\s_t\subset \M, |\s_t|<\infty,\\
        &\text{(At each time step, the system's reservoir of options }\\
        &\text{expands with new options.)}\\
        &\exists C>0, \text{ s.t. } \theta_t(a)<C, \text{ for }\forall a\in\s_t\setminus\s_{t-1},\\
        &\text{(Model estimates for unseen new options are bounded.)}
        \end{flalign*}
    \item New conditions in Theorem~\ref{thm:s4_suff}:
        \begin{flalign*}
        &c^i_t(a) = 1: \theta^j_{t+1}(a) > \theta^j_t(a) \text{ for } \forall j\in[n] \text{ s.t. } d(\mu^i_t, \mu^j_t) < \epsilon,\\
        &c^i_t(a) = 0: \theta^j_{t+1}(a) < \theta^j_t(a) \text{ for } \forall j\in[n] \text{ s.t. } d(\mu^i_t, \mu^j_t) < \epsilon,\\
        &\text{(An engaged option increases model estimate of similar users'}\\
        &\text{corresponding model parameter, and vice versa.)}\\
        &|\theta^i_{t+1}(a^{l, i}_t) - \theta^i_t(a^{l, i}_t)| > \sum_{u\in\U_i} |\theta^i_{t+1}(a^{l', u}_t) - \theta^i_t(a^{l', u}_t)| \\
        &\text{ for } l,l'\in[k]. \\
        &\text{(Direct feedbacks result in more significant model updates}\\
        &\text{than drawing inferences from similar users.)}
        \end{flalign*}
\end{enumerate}

\end{appendices}
